# Supplementary material for: Reference Capabilities for Flexible Memory Management: Extended Version
Source: arXiv:2309.02983 ancillary file (2023-09-06)

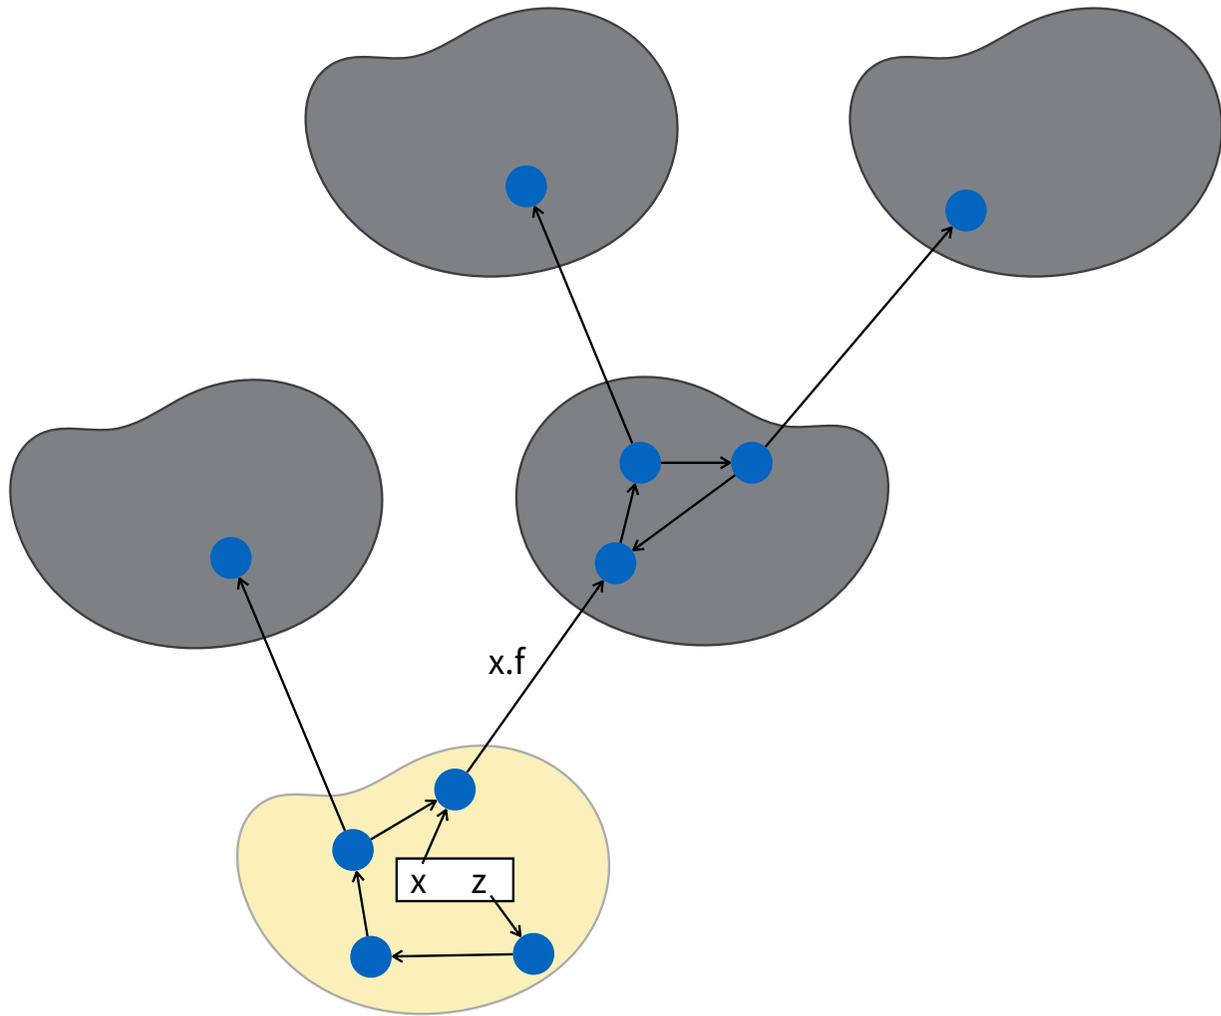

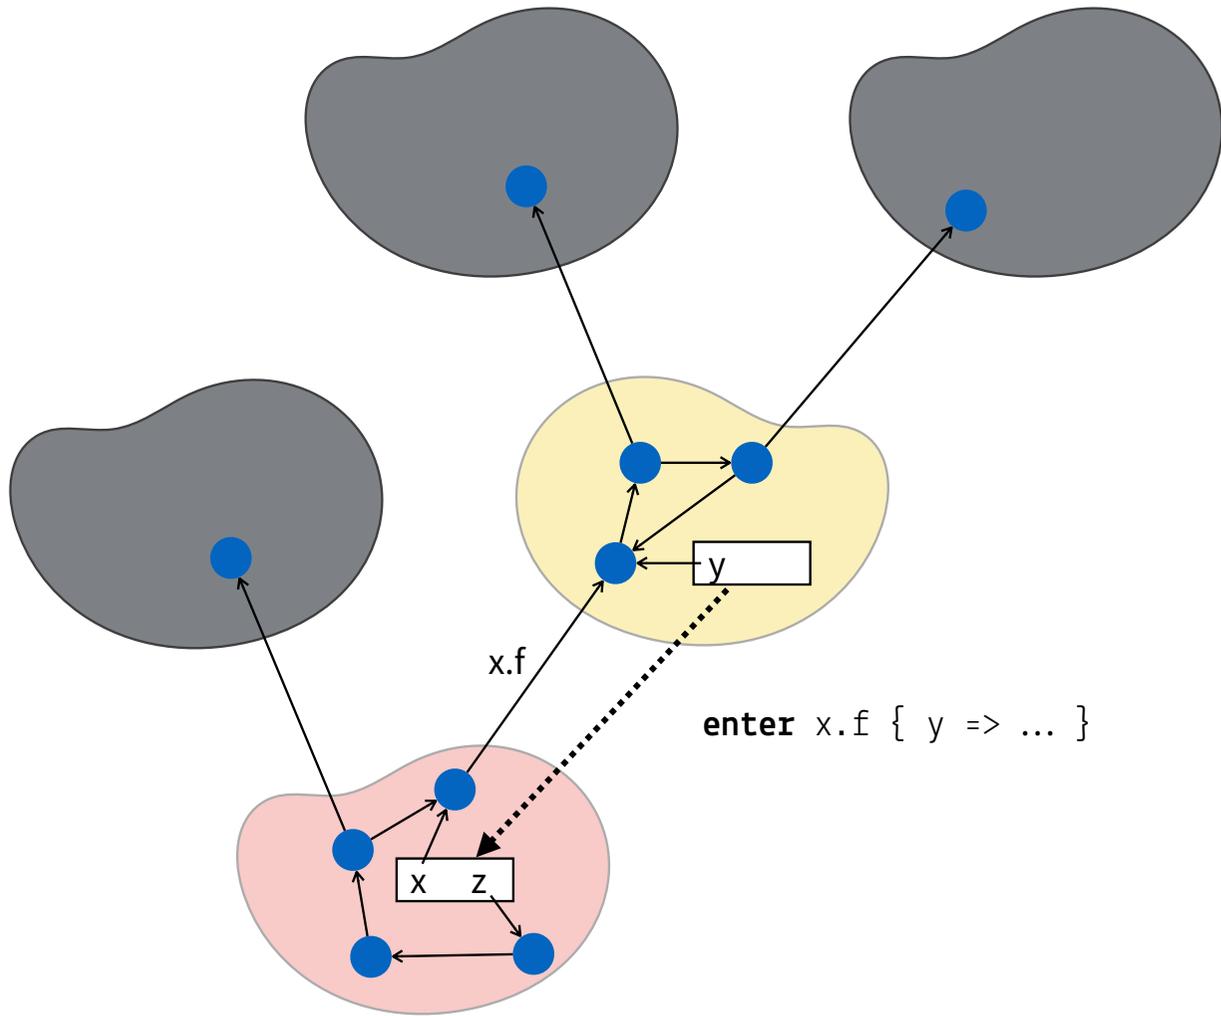

Supplement: Supplementary file 1 [file figures.pdf]
