# Supplementary material for: Reference Capabilities for Flexible Memory Management: Extended Version
Source: arXiv:2309.02983 ancillary file (2023-09-06)

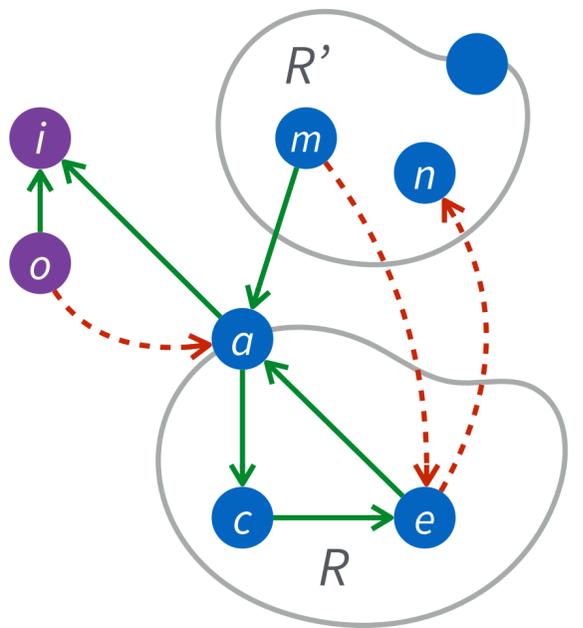

● immutable ← OK  
● mutable ← Not OK

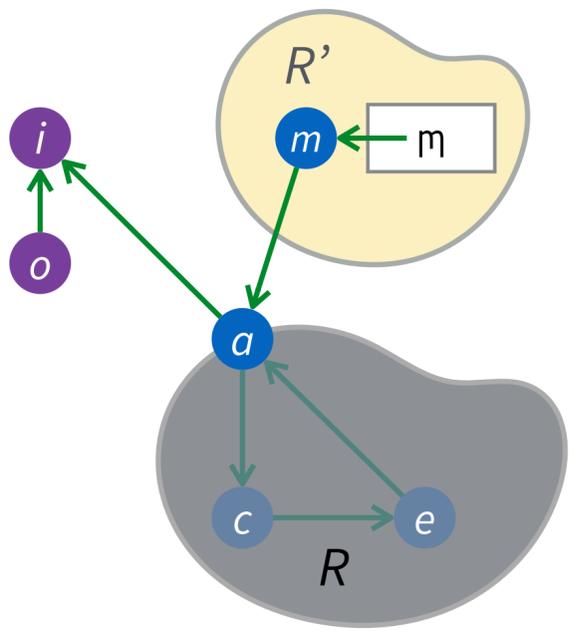

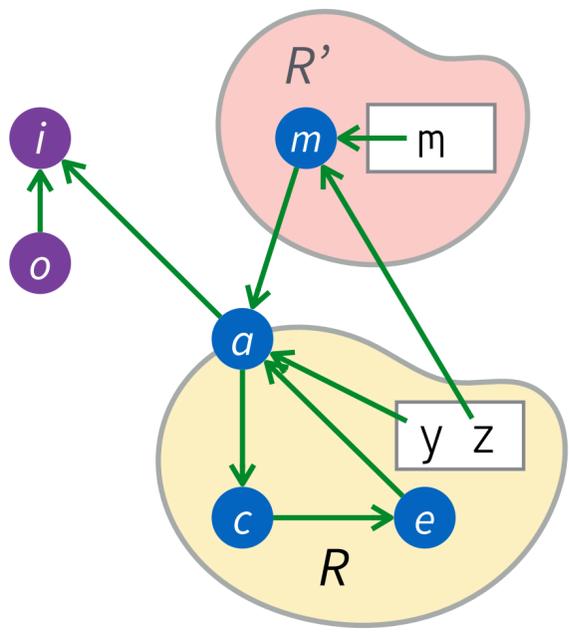

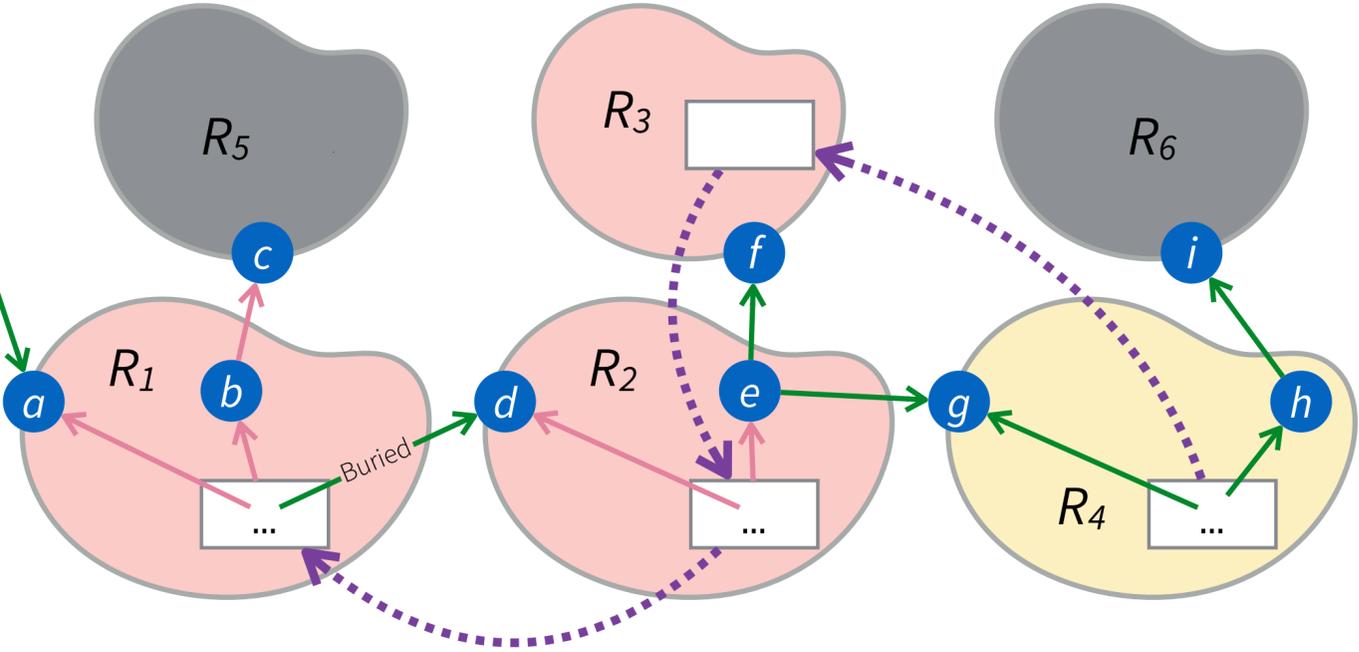

- ← **paused** ref
- ← **mut/iso** ref
- ◡ paused ( $R_{1,2,3}$ )
- ◡ active ( $R_4$ )
- ◡ closed ( $R_{5,6}$ )
- enter** block scope
- ⋯← region LIFO order

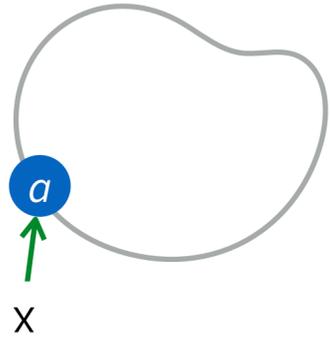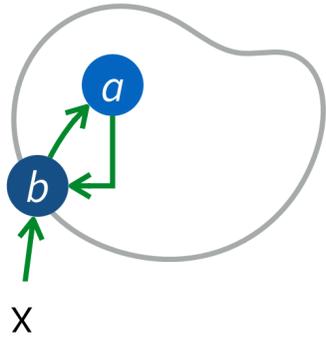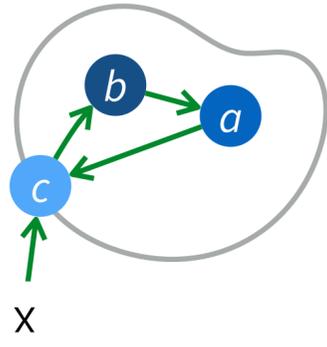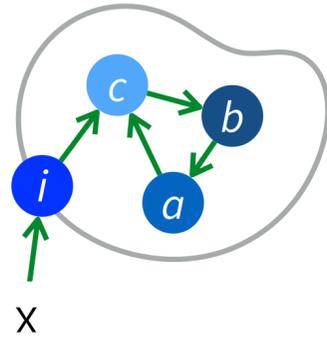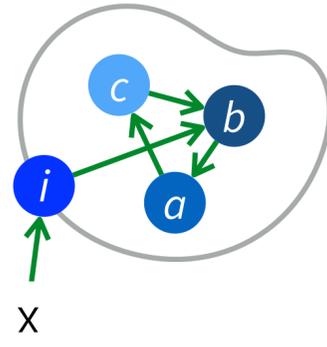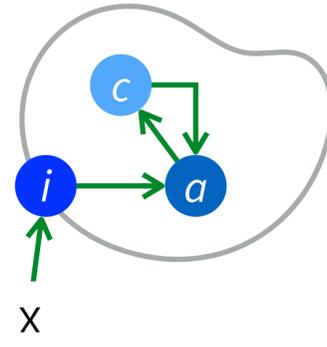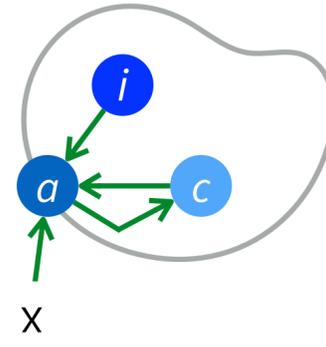

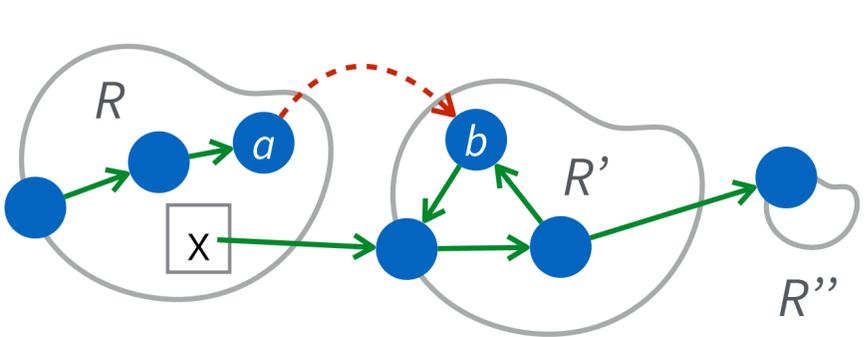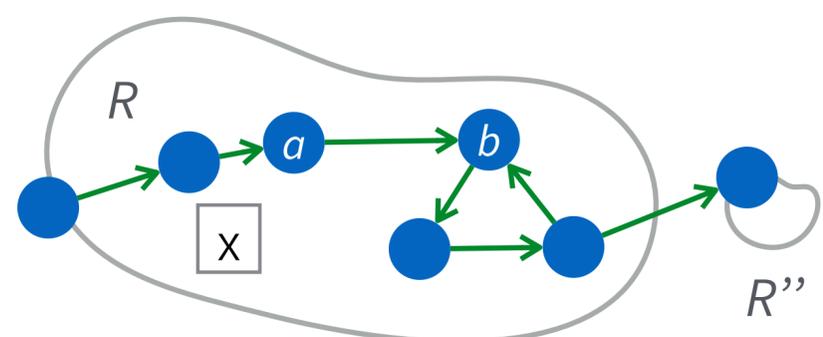

merge  $R'$  into  $R$  —  $R''$  is unaffected

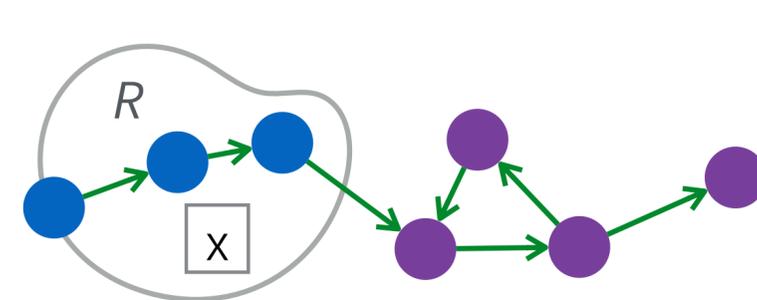

freeze  $R'$  also freezes  $R''$

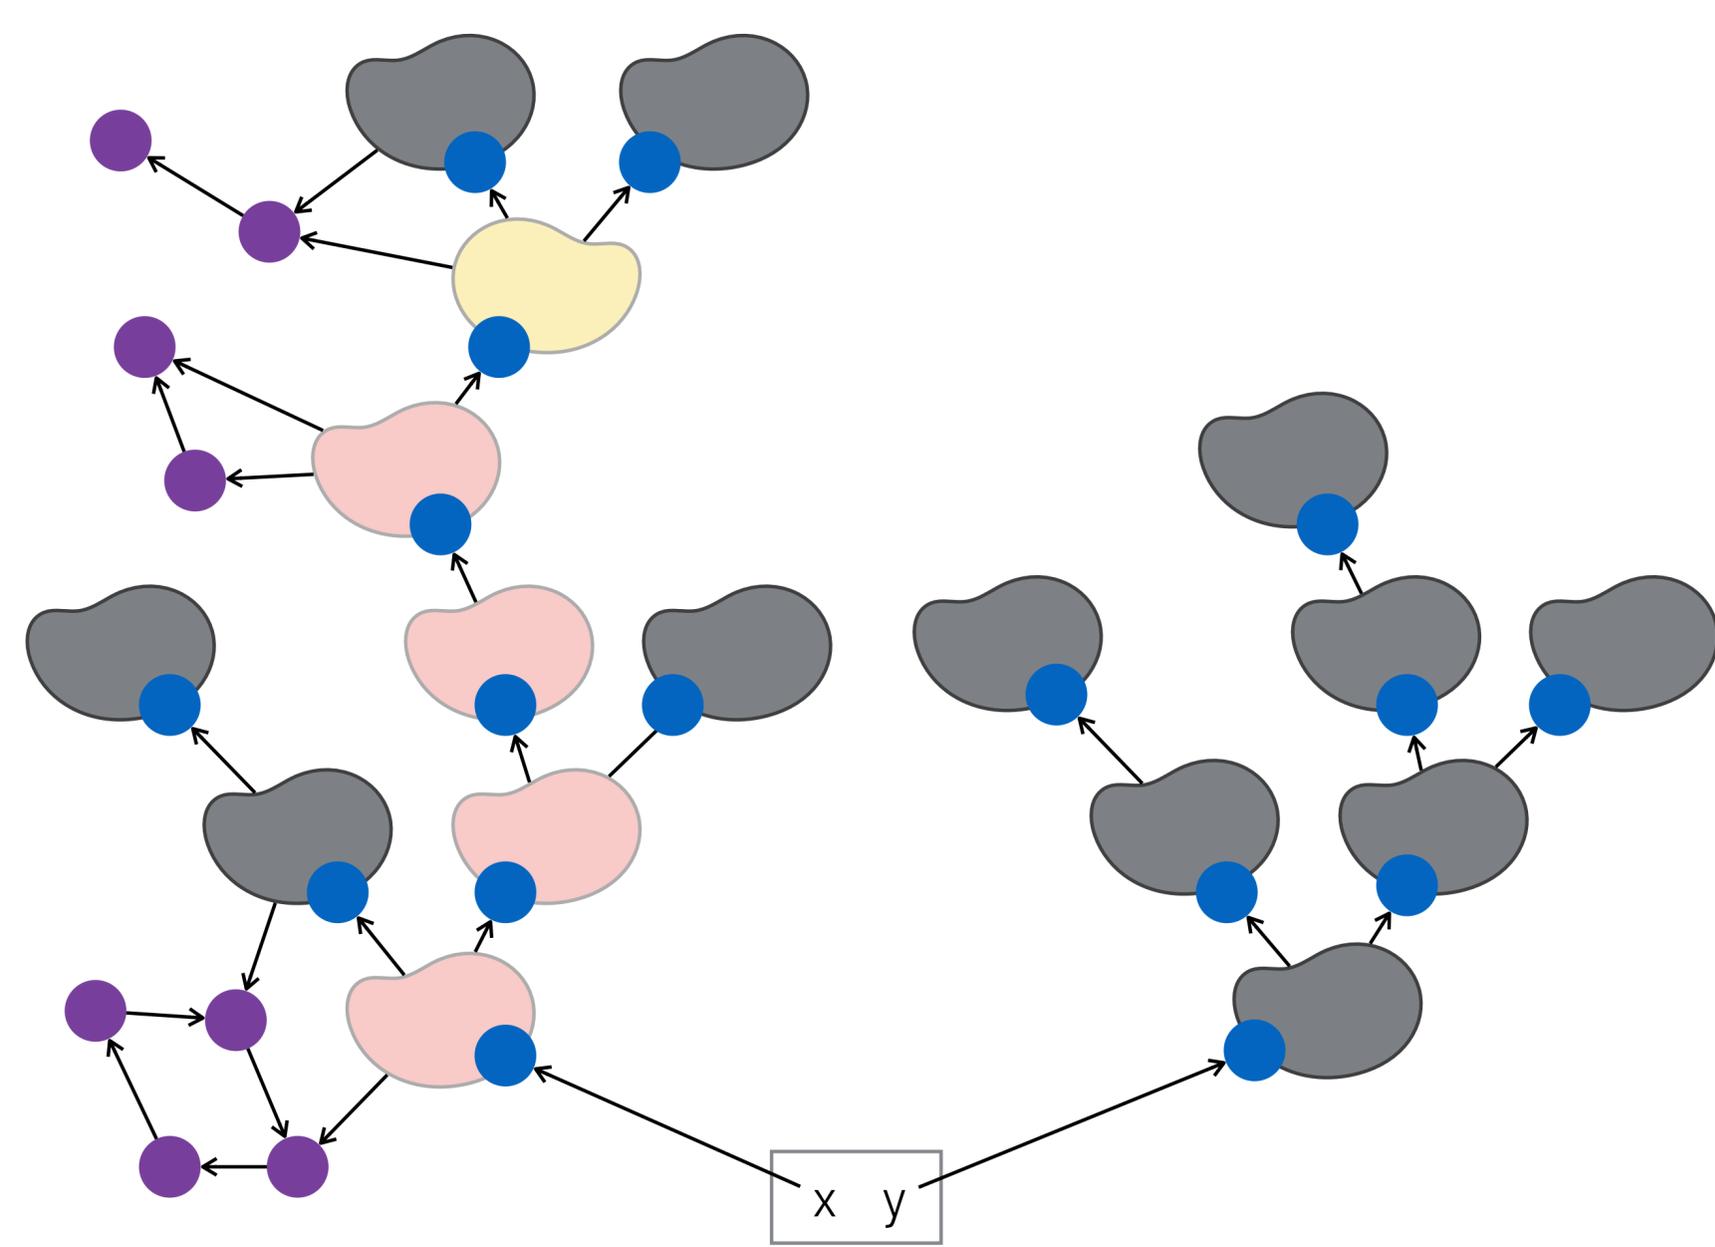

```
enter x as x => [y] {  
  enter y as y => {  
    let a = new (x & y) Foo  
    enter y.f as z z => {  
      some_function[x](x);    // x : tmp & Store[x & Bar]  
      some_function[x, y](a); // a : x & y & Foo  
      some_function[x, z](z); // z : z & Baz  
    }  
  }  
}
```

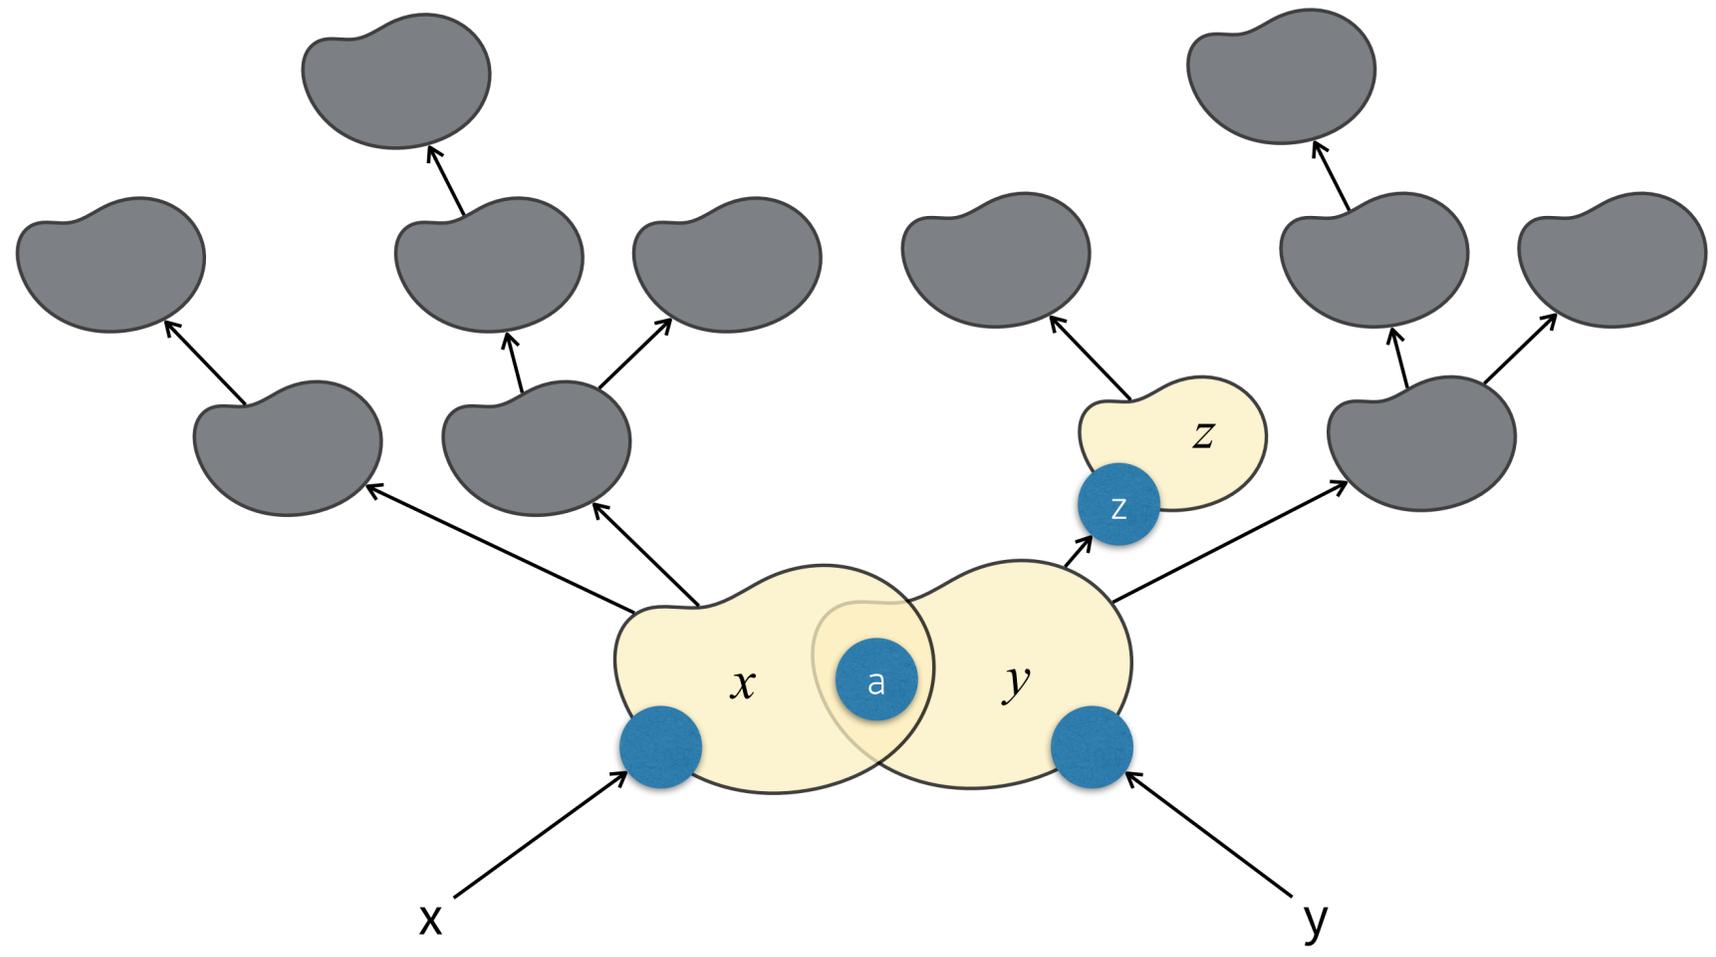

```
enter x as x => [y] {  
  enter y as y => {  
    let a = new (x & y) Foo  
    enter y.f as z z => {  
      some_function[x](x);    // x : tmp & Store[x & Bar]  
      some_function[x, y](a); // a : x & y & Foo  
      some_function[x, z](z); // z : z & Baz  
    }  
  }  
}
```

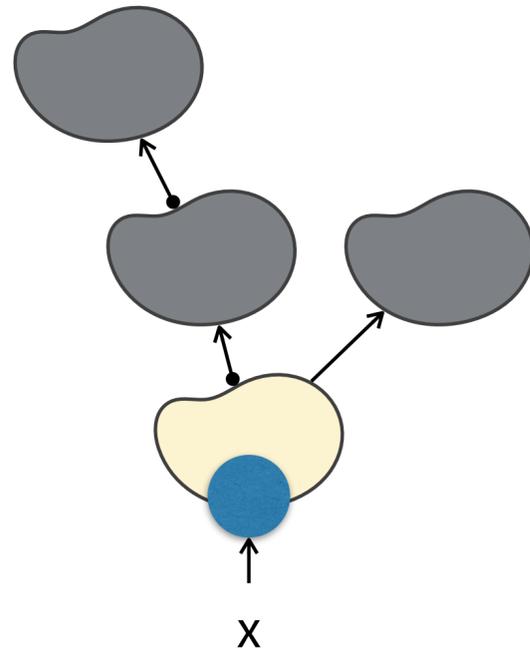

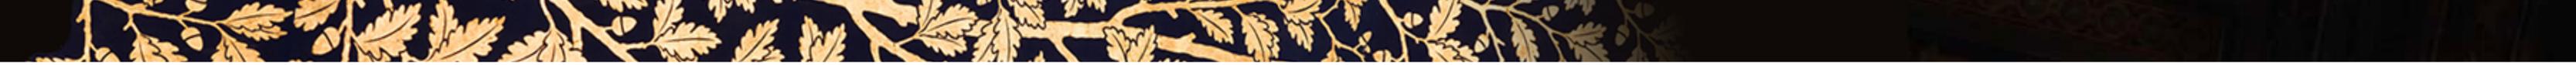

# Type System Design Goals wrt Concurrency and Memory Management

---

## Safe Concurrency

Data-race freedom — if two behaviours simultaneously have access to an object, both consider it immutable

## Mix-and-Match Memory Management

A region is free to manage its own memory in “whatever” way it likes, irrespective of all other regions in the program

## Incremental Memory Management

We can determine liveness in the active region without worrying about/or tracking pointers or liveness of objects in any other region

## Concurrent Memory Management

A behaviour can mediate between program work or memory management work without informing or synchronising with other behaviours

## Local Reasoning about Memory Management Costs

**The cost of managing the memory of the active region is a function of the activities/objects/pointers in the active region only**

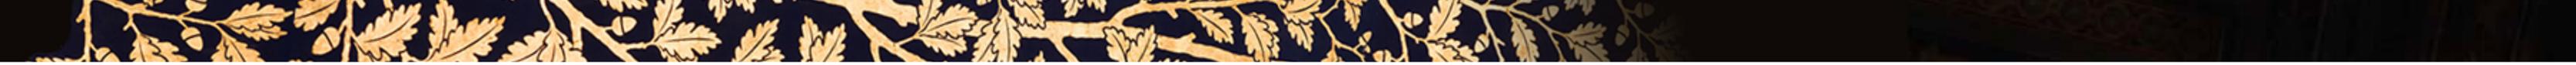

# What the Type System Adds

---

## **Full Encapsulation of Regions**

If object A points to and can mutate object B, then A and B are in the same region

## **External Uniqueness of Bridge Object**

A bridge object to a region R has at most one incoming pointer from objects external to R

## **Single Mutable Region**

Each behaviour holds a LIFO stack of the currently open regions in the order of their opening; only the top-most region is mutable ; all behaviour's region stacks are disjoint

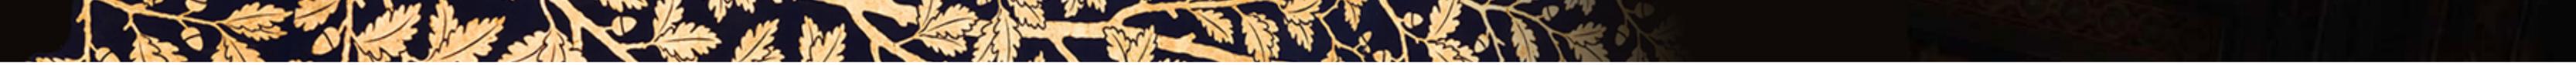

Is anything  
missing?

# Fill in the Table

---

|                  | Full encapsulation | External Uniquess | Single Mutable Region |
|------------------|--------------------|-------------------|-----------------------|
| Safe concurrency |                    |                   |                       |
| Mix-and-Match    |                    |                   |                       |
| Incremental      |                    |                   |                       |
| Concurrent       |                    |                   |                       |
| Local Reasoning  |                    |                   |                       |

# Fill in the Table

|                  | Full encapsulation | External Uniqueness | Single Mutable Region |
|------------------|--------------------|---------------------|-----------------------|
| Safe concurrency | 👍                  | 👍                   |                       |
| Mix-and-Match    | 👍                  |                     |                       |
| Incremental      | 👍                  |                     |                       |
| Concurrent       | 👍                  | 👍                   |                       |
| Local Reasoning  |                    |                     | 👍                     |

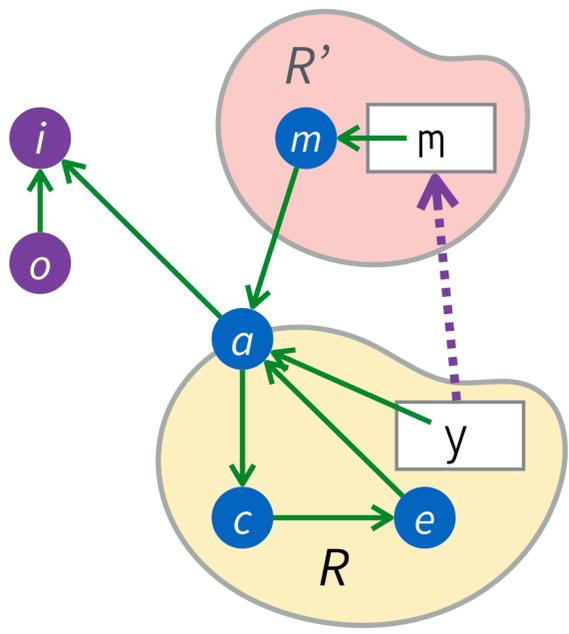

Supplement: Supplementary file 2 [file popl22-figures.pdf]
